# Supplementary material for: TRILLsson: Distilled Universal Paralinguistic Speech Representations
Source: arXiv:2203.00236 source file (2022-03-20)
Supplement: Supplementary file 1 [file 6_appendix.tex]

\begin{centering}
\begin{table*}[t]
\scriptsize
\vspace{-0.2cm}
%\caption{Accuracies (\%) for NOSS tasks. }
\caption{d-prime results.
}\label{tab:dprime}

\centering
\begin{tabular}{@{} llcc|c|cccccc @{}}
\toprule[2pt]
\begin{tabular}{@{}c@{}}Model\\(input)\end{tabular} &
Arch. &
\begin{tabular}{@{}c@{}}Params\\ (M)\end{tabular} &
\begin{tabular}{@{}c@{}}Size\\ (MB)\end{tabular} &
\begin{tabular}{@{}c@{}}Avg D-\\Prime\end{tabular} &
Voxforge* & 
\begin{tabular}{@{}c@{}}Speech \\ Commands\end{tabular}   &  
\begin{tabular}{@{}c@{}}ASVSpoof\\ 2019\end{tabular} & 
Euphonia* &
CREMA-D &
IEMOCAP
\\
\toprule[2pt]
\textbf{CAP12} \\
% Architecture avg test voxforge speechcommands maskchallenge asvspoof euphonia cremad iemocap params size 
\quad (full)  & \scriptsize{Conformer}
& 606 & 2,200 & 2.99  & 5.39 & 4.66 & 1.02 & 3.53 & 1.18  & 3.05 & 2.08  \\
\quad (3sec) & \scriptsize{Conformer}
& 606 & 2,200 & 2.93  & 5.13 & 4.64 & 1.02 & 3.53 & 1.12  & 3.05 & 2.01  \\
\quad (2sec) & \scriptsize{Conformer}
& 606 & 2,200 & 2.80  & 5.11 & 4.65 & 1.02 & 2.96 & 1.04  & 2.91 & 1.93  \\
\midrule
\textbf{Public} \\
\textbf{Baselines} \\
% voxceleb voxforge speechcommands maskchallenge asvspoof euphonia cremad iemocap 
\quad Wav2Vec2  & Transformer 
& ? & ? & ?  & ? & ? & ? & ? & ? & ?  & ? \\
\quad TRILL     & Resnetish 
& 24.5 & 86.6 & 1.89 & 2.40  & 2.94 & 0.78 & 2.96 & 0.86 & 1.95  & 1.35 \\
\quad YAMNet     & Resnetish
& 3.7 & 17.0 & 1.79  & 2.08 & 3.11 & 0.49 & 2.94 & 0.67  & 1.92 & 1.35  \\
\midrule
\textbf{TRILLsson} \\
% voxceleb voxforge speechcommands maskchallenge asvspoof euphonia cremad iemocap 
\quad 5 (2sec) & \scriptsize{AST} % ast_sec3_l12_m2048,48000,tr=False
& 88.7 & 340 & ?  & ? & ? & ? & ? & ?  & ? & ?  \\
\quad 4 (2sec) & \scriptsize{AST} % ast_sec2_l12_m512,32000,tr=False
& 50.8 & 196 & ?  & ? & ? & ? & ? & ?  & ? & ?  \\
\quad 3 (2sec) & \scriptsize{E.NetV2} % efficientnetv2bS,32000,tr=False	
& 21.4 & 95 & ?  & ? & ? & ? & ? & ?  & ? & ?  \\
\quad 2 (2sec) & \scriptsize{E.Net} % efficientnetb3,32000,tr=False	
& 12.2 & 57 & ?  & ? & ? & ? & ? & ?  & ? & ?  \\
\quad 1 (2sec) & \scriptsize{Resnetish} % resnetish_sec3_2352_0.5,48000,tr=False
& 5.0 & 22 & ?  & ? & ? & ? & ? & ?  & ? & ?  \\
\quad 0 (2sec) & \scriptsize{Resnetish} % resnetish_sec3_2352_0.25,48000,tr=False	
& 1.2 & 6.4 & ?  & ? & ? & ? & ? & ?  & ? & ?  \\
\bottomrule
\end{tabular}
\end{table*}
\end{centering}
